# Supplementary material for: Refining Machine Learning Potentials through Thermodynamic Theory of Phase Transitions
Source: arXiv:2512.03974 ancillary file (2025-12-03)
Supplement: Supplementary file 1 [file supplementary_information.pdf]

# Supplementary Information

## Refining Machine Learning Potentials through Thermodynamic Theory of Phase Transitions

Paul Fuchs[1] and Julija Zavadlav[1,2*]

[1]Professorship of Multiscale Modeling of Fluid Materials, Department of Engineering Physics and Computation, TUM School of Engineering and Design, Technical University of Munich, Germany.
[2]Atomistic Modeling Center (AMC), Munich Data Science Institute (MDSI), Technical University of Munich, Germany.

*Corresponding author(s). E-mail(s): julija.zavadlav@tum.de;

## Supplementary Note 1: Pretraining with Force Matching

We pretrain a MACE [1] model using the hyperparameters listed in Table 1. Therefore, we minimize the force-matching loss in 400 epochs with a batch size of 16 using the ADAM optimizer [2] with weight decay of $1e^{-2}$, $\beta_1 = 0.95$, $\beta_2 = 0.995$, and exponential learning rate decay from $3e^{-3}$ to $3e^{-6}$. For the loss coefficients, we choose $\gamma_u = 1e^{-5}\text{kJ}^{-2} \cdot \text{mol}^2$, $\gamma_{\mathbf{f}} = 1e^{-2}\text{kJ}^{-2} \cdot \text{mol}^2 \cdot \text{nm}^2$, and $\gamma_\sigma = 4e^{-6}\text{kJ}^{-2} \cdot \text{nm}^6$. We monitor convergence by empirically estimating the loss on a disjoint validation split and select the parameterization $\theta$ that yields the lowest error on the validation split.

**Supplementary Table S1**: MACE Hyperparameters

| Hyperparameter | Value | Hyperparameter | Value |
|---|---|---|---|
| Cutoff | 0.5 nm | Hidden Irreps | $64 \times 0e + 32 \times 1o$ |
| Readout Irreps | $16 \times 0e$ | Interaction Irreps | O3-Restricted |
| Max. $\ell$ | 3 | Interaction Layers | 2 |
| Correlation Order | 3 | Radial Basis Dim. | 8 |
| Polynomial Envelope Degree | 6 | | |

## Supplementary Note 2: DiffTTC Optimization

We correct the transition temperature using the DiffTTC temperature of a pretrained potential. Therefore, we determine the DiffTTC optimization target using preparatory simulations, including coexistence simulations and free energy integrations as described in Supplementary Notes 3 and 4. We then refine the model parameters for 250 epochs using the DiffTTC method with a batch size of 6. Therefore, we set up simulation boxes using the density and lattice constants determined in Supplementary Information 4. For the BBC and liquid systems, we obtain the boxes through replicating a BCC unit cell $6 \times 6 \times 8$ times. For the HCP systems, we replicate the HCP unit cell $9 \times \times 4 \times 4$ times. Therefore, the boxes contain the same number of atoms and have an approximately equal spatial extent. We use a Nosé-Hoover thermostat with coupling constant of 2 ps to run simulations at the target temperatures, where we equilibrate the system for 20 ps and collect samples every 0.5 ps within 100 ps. We optimize the model parameters using the ADAM optimizer [2] with $\beta_1 = 0.9$, $\beta_2 = 0.99$, combined with an exponential learning rate decay from $5 \cdot 10^{-5}$ to $5 \cdot 10^{-6}$. Additionally, we employ a weight decay with a strength of $10^{-2}$ to restrain the model parameters to the pretrained parameters $\theta_0$.

Figure 1 displays the optimization loss and the gradient norm. In the initial epochs, the loss decays quickly. In the following epochs, the loss decreases much more slowly, reaching a value of around 0.024 after 200 epochs, which does not significantly improve until the end of the optimization.

We verify the consistency of the free energy estimates in training by comparing them to predictions obtained using non-equilibrium thermodynamic integration and the coexistence method. Therefore, we

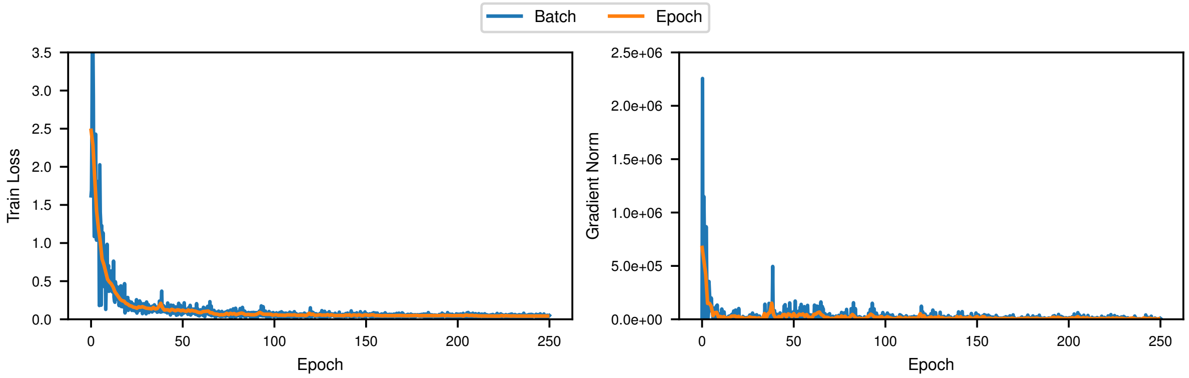


**Supplementary Figure S1**: **Loss and Gradient Norm during the DiffTTC optimization.** The optimization starts from the pretrained MLP for Titanium and contains 24 statepoints. The first 12 statepoints correspond to 6 HCP-BCC transitions at equally spaced pressures from 0 to 5 GPa. The other 12 statepoints correspond to 6 BCC-liquid transitions at equally spaced pressures from 0 to 5 GPa.

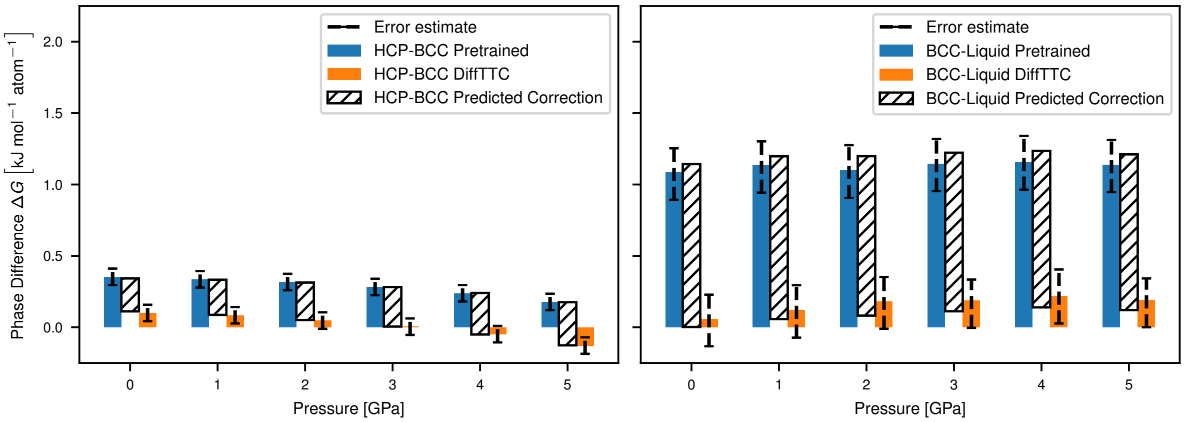


**Supplementary Figure S2**: **Free Energy Differences between Phases**: Predictions for the pretrained and refined model at the experimentally determined coexistence temperatures and pressures. The shaded areas correspond to the free energy difference estimated by the trainer. The error bars correspond to the linearly extrapolated change in free energy due to varying the coexistence temperature (zero free energy difference) by +5 K.

the coexistence method followed by Reversible Scaling for the BCC-Liquid transition as described in Supplementary Notes 3 and 4. Supplementary Figure 2 shows the free energies predicted during and outside of training in comparison to approximate error estimates (see Supplementary Note 5). In general, the free energy differences computed sequentially during the DiffTRe optimization are consistent with the values outside training within the estimated error magnitudes. However, the estimated errors and also the deviation between the predicted values are higher for the BCC-liquid phase transition than for the HCP-BCC transition. This difference in consistency between the two transitions might arise due to the more involved free energy integration for the former. The estimated temperature in the coexistence method is uncertain due to temperature fluctuations that might only be resolved during long simulation times (see Supplementary Notes 5). However, even small uncertainties around 5 to 10 K can affect the free energy in the order of 1 meV atom$^{-1}$. Additionally, the Reversible Scaling method requires significantly longer simulation times than the Frenkel-Ladd path to reach the same accuracy, especially when the predicted coexistence temperature of the prior potential necessitates integration over large temperature ranges. Potentially, these errors can be avoided by the free energy integration method acting directly at the target temperature, such as the Pseudo-Critical Path Method [3].

## Supplementary Note 3: Coexistence Simulations

To estimate the BCC-liquid coexistence temperatures, we perform simulations with solid-liquid coexistence [6] at multiple initial temperatures and run isobaric-isoenthalpic (NPH) simulations until the average amount of BCC crystal structure remains constant.

To prepare two interfaces perpendicular to the $x$ axis, we create a BCC supercell with $30 \times 15 \times 15$ ($30 \times 10 \times 10$ for the MACE-MP-0b3 model) unit cell repetitions in the $x$, $y$, and $z$ directions. We couple the system to a barostat with coupling constant of 1 ps, which scales the box independently in the $x$ direction and jointly in the $y$ and $z$ directions. To create a distinct liquid and solid region, we define two Langevin thermostats with coupling constants of 0.1 ps. The first thermostat corresponding to the liquid region is coupled to

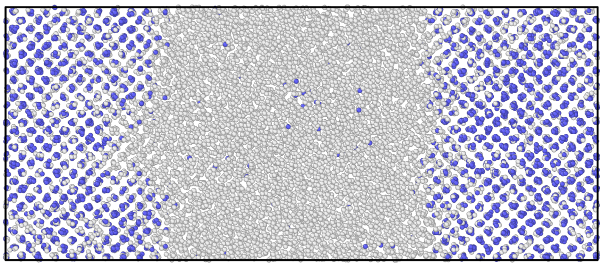

**Supplementary Figure S3**: **Solid-Liquid Coexistence** Equilibrated system of titanium with coexistence of solid (BCC) and liquid phase. The particles are colored in blue if assigned to a BCC local structure via the Polyhedral Template Matching method [4] and colored white otherwise. Visualized in ovito [5].

all particles $i$ with $x_i \in [0.3L_x, 0.7Lx]$, where $L_x$ is the box-length in the $x$ direction. The second thermostat corresponding to the solid region is coupled to the remaining particles. First, we run a 4 ps simulation, where we heat the liquid region to 700 K above the estimated melting temperature, while cooling the solid region to 300 K below the estimated melting temperature. Then, we linearly ramp both thermostats to the predicted melting temperature within a 2 ps simulation. Finally, we decouple the local Langevin thermostats and add a global Nosé-Hoover thermostat with coupling constant of 0.4 ps to perform another short 2 ps simulation at the estimated melting temperature.

After the preparatory simulations, we obtain a solid-liquid coexistence at a homogeneous temperature but not in equilibrium. Thus, we decouple the thermostat from the system to allow the temperature to vary and run an NPH simulation for 160 ps. During the simulation, parts of the liquid should solidify, or parts of the solid should melt, until the coexistence temperature is reached. Therefore, we monitor the temperature and the average fraction particles with BCC crystallinity using the Polyhedral Template Matching method [4] with RMSD of 0.18 $Å^2$. If the fraction remains approximately constant, we calculate the melting temperature as the average of the recorded temperatures. Otherwise, we repeat the preparation, adjusting the estimated melting temperature accordingly.

## Supplementary Note 4: Free Energy Computations

We employ the Frenkel-Ladd approach to calculate the reference free energies for the HCP and BCC phases at a given temperature. However, the Einstein Crystal potential describes a system of independent particles, such that we cannot define a pressure [7]. Thus, we integrate the Helmholtz free energy using non-equilibrium thermodynamic integration in the NVT ensemble [7] and compute the Gibbs free energy via $\Delta G^{\mathrm{I}\to\mathrm{II}} = \Delta F^{\mathrm{I}\to\mathrm{II}} + P\Delta V^{\mathrm{I}\to\mathrm{II}}$.

To set up the NVT simulations, we compute the lattice constants and molar volumes in preparatory simulations at the target pressure and temperature. Moreover, we determine the mean-squared particle displacement $\bar{\Delta} = \langle(\Delta r)^2\rangle$ to compute the Einstein Crystals' spring constants via $k = 3k_BT/\bar{\Delta}$ following Freitas et al. [7]. For the preparatory simulations, we replicate BCC unit cells $16 \times 16 \times 16$ for the BCC and liquid states and HCP unit cells $20 \times 10 \times 10$ times for the HCP states to obtain initial boxes. We couple these boxes to Langevin thermostats with coupling constants of 0.1 ps and Nosé-Hoover barostats with coupling constants 4.0 ps, where the box scales isotropically in all dimensions for the BCC and liquid systems and independently in $z$ direction for the HCP systems. Before performing simulations at the experimentally determined transition temperatures and pressures, we superheat the liquid systems to a temperature 1000 K higher than the target temperature, and linearly ramp the temperature to the target temperature within 8 ps. Following, we equilibrate all systems for 8 ps and write out lattice parameters and mean-squared particle displacements every 10 time steps during 40 production simulations.

For the Frenkel-Ladd integration, we then use the average lattice parameters obtained from preparatory simulations and replicate BCC unit cells $16 \times 16 \times 16$ for the BCC and liquid states and HCP unit cells $20 \times 10 \times 10$ times for the HCP states to create initial boxes with correct dimensions. We run the integrations at the experimentally determined HCP-BCC coexistence temperatures using Langevin thermostats with coupling constants of 0.1 ps and zero net random force. We equilibrate the system for 4 ps, then run the forward integration within 20 ps, equilibrate again for 4 ps, and perform the backward integration within 20 ps. We write out the potential energy of the system at every time step.

Finally, we use the Reversible-Scaling method to calculate the change in free energies with temperature, while maintaining constant pressure, for both solid and liquid phases. To reduce equilibration time, especially for the liquid system, we start the integration from reference boxes created during the preparatory simulations. We perform NPT simulations at the experimentally determined coexistence temperatures and pressures using Nosé-Hoover thermo- and barostats with coupling constants of 0.4 ps and 4.0 ps, respectively. For the BCC and liquid systems, we couple all dimensions to the same barostat. For the HCP system, two barostats are applied independently, one for the $x$ and $y$ dimensions and one for the $z$ dimension. We equilibrate for 4 ps, then perform the forward integration in 40 ps, equilibrate again for 4 ps, and finally perform the backward integration in 40 ps time.

## Supplementary Note 5: Error Estimates

For the free-energy integrations, we estimate our errors based on the study of Freitas et al. [7], which analyzes the error contributions through finite system sizes and integration time. Table 2 summarizes the characteristic scale and the corresponding error estimate.

**Supplementary Table S2**: **Error Estimates for Free Energies.** The errors are approximated by comparing system size and integration rate to errors reported in Freitas et al. [7]. The integration rate in the reversible scaling simulation is lower for the DiffTTC model with improved temperature than for the pretrained model, as a smaller temperature range must be swept.

| **Method** | | **Critical Quantity** | **Error** (meV atom$^{-1}$) |
|---|---|---|---|
| **Reversible Scaling** | | | |
| System Size | (atoms) | $\sim 8 \cdot 10^3$ | $0.3^+$ |
| Integration Rate | (K step$^{-1}$) | $< 3.5 \cdot 10^{-2}$ / $< 1.75 \cdot 10^{-2*}$ | 1 / 0.5 |
| **Frenkel Ladd** | | | |
| System Size | (atoms) | $\sim 8 \cdot 10^3$ | $0.3^+$ |
| Integration Time | (K step$^{-1}$) | 5000 | $< 0.02$ |

$^*$ DiffTTC model

$^+$ Reported for the combination of Frenkel-Ladd and Reversible Scaling path

We propagate the uncertainty in the free energy computations to get a rough estimate of the uncertainty in the HCP-BCC transition temperature. Therefore, we shift the free energy profiles obtained by the Frenkel-Ladd and Reversible Scaling method by 2 meV atom$^{-1}$ for the pretrained model and 1 meV atom$^{-1}$ for the DiffTTC model closer together to account for the integration time error in the HCP and BCC free energy profiles. We use the obtained change in temperature as the error estimate for the transition temperature.

Similarly, we compute a temperature error in the coexistence method. Therefore, we assess the convergence and error of the temperature through a block error analysis. In this analysis, we divide the trajectory into $K \geq 4$ equally sized blocks and compute the block means $\bar{T}_k$. We then estimate the standard deviation $\sigma_T(\bar{T}_k)$ of the block means to compute the standard error of the total mean via $s_K(T) = \sigma_T(\bar{T}_k)/\sqrt{K}$. Figure 4 displays the standard error and the block standard deviation against the block size. As the block standard deviation is not fully converged, we assume a 50 % higher value of the standard error. We then set the error of the coexistence method equal to twice the estimated standard error, i.e., $\Delta T = 3s_K(T)$, which is around 5 K on average.

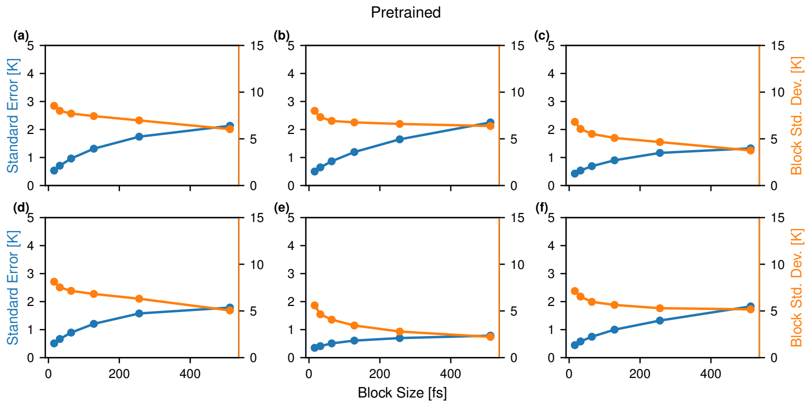


**Supplementary Figure S4**: Block error analysis of the temperature in the coexistence simulation using the pretrained model. The plots show the standard deviation of the block means against the block size (orange) and the standard error of the total block mean (blue).

We also propagate the error in the coexistence temperature to the free energy error between BCC and liquid phase. Therefore, we approximate the change of free energy per temperature $\frac{dF}{dT} \approx \frac{\Delta F}{\Delta T}$ by shifting the intersection of the free energy profiles obtained through Reversible Scaling simulations to a $\Delta T = 5\ K$ higher temperature. We then use this slope to interpolate the free energy error based on the temperature as described in the previous section.

## Supplementary Note 6: Computation of Volumes, Radial and Angular Distribution Function, and Diffusion Coefficient

We calculate the lattice constants and volumes using short molecular dynamics simulations at zero pressure. To reduce the equilibration times, we start the simulation at the highest temperatures, starting from the equilibrated box used for the non-equilibrium free energy computations (see Supplementary Note 4). We use Nosé-Hoover barostats with coupling constants of 1.0 ps, where all directions for the BCC and liquid systems, as well as the $xy$ direction for the HCP system, are coupled to the same barostat. To maintain the temperature, we employ a Langevin thermostat with coupling constant of 0.1 ps. We first equilibrate the systems at the target temperature in a short 5 ps simulation. Then, we collect volume and lattice constants every 10 frames in a 20 ps simulation. Additionally, we write out the trajectory every 100 frames. We repeat the equilibration and production simulations for the lower temperatures, starting the equilibration at the last frame of the previous production run.

Using the liquid trajectory at a given temperature, we calculate the radial and angular distribution functions as averages over their instantaneous values at every collected time step. For the angular distribution function, we select 0.0 nm as inner cutoff and the first solvation shell, computed as the first minima from the radial distribution function, as the outer cutoff.

We compute the diffusion constants via two typically employed approaches [8]. In the Green-Kubo relations, the diffusion constant is proportional to the integral of the velocity autocorrelation function

$$D = \frac{1}{3} \lim_{t\to\infty} \int_0^t \frac{1}{N} \langle \boldsymbol{v}(0) \cdot \boldsymbol{v}(t) \rangle dt. \tag{1}$$

In the Einstein relation, the mean-squared particle displacement asymptotically converges towards a linear relation with time, with slope given by the diffusion constant

$$D = \frac{1}{6} \lim_{t\to\infty} \frac{1}{N} \langle \|\boldsymbol{r}(0) - \boldsymbol{r}(t)\|^2 \rangle. \tag{2}$$

Thus, we run simulations to compute the velocity autocorrelation function and the mean-squared displacement of the particles over time.

For both simulations, we replace the Langevin thermostat used in the previous simulations with a Nose-Hoover thermostat with a coupling constant of 0.1 ps to avoid erroneous dynamics. Moreover, we start both simulations at the last frame with the corresponding temperature from the previous volume computation. For the velocity autocorrelation function, we first equilibrate the thermostat for 1 ps. Then, we reduce the timestep by a factor of 8 to increase the resolution of the function and collect the correlation of the current velocity with the initial velocity for 0.5 ps. For each temperature, we only collect a single sample. However, the large number of 8192 particles and the repetitions for 12 different temperatures result in a linear fit over temperature with adequate uncertainty (see Figure 5).

For the mean-squared displacement approach, we similarly equilibrate the thermostat for 1 ps and then collect the mean-squared particle displacement to the current position in a 4 ps simulation. We compute the diffusion constants via a linear fit to the mean squared displacement after 2 ps. The uncertainty of the estimates is smaller due to the longer simulation time. However, the estimates deviate towards higher diffusion values. This deviation may be attributed to a bias that arises from unwrapping the displacement in a system with a barostat [9]. Thus, we only consider the diffusion samples computed via the velocity-autocorrelation function approach in the computation of the diffusion versus temperature fit.

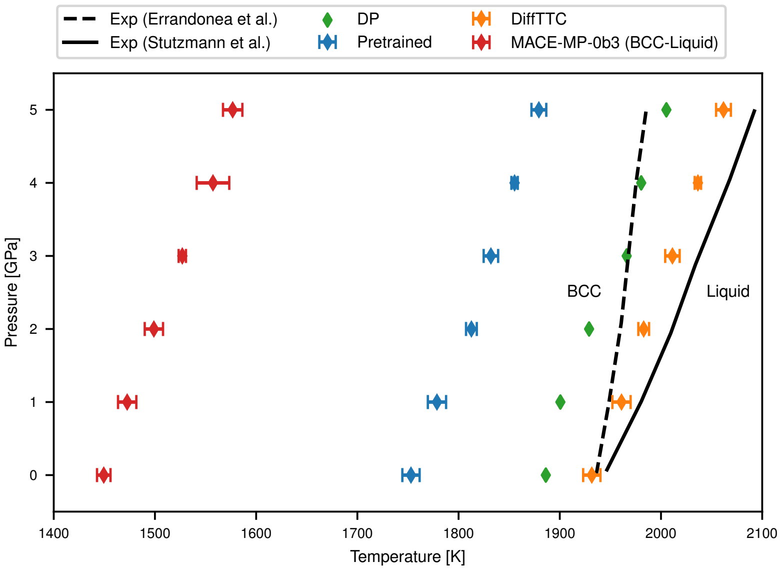


**Supplementary Figure S5**: Melting Temperatures of Titanium predicted by the pretrained and DiffTTC-refined MLP in comparison to predictions of the foundational MACE-MP-0b3 [10] model, values for the DP potential from Wen et al. [11] and experimental data from Errandonea et al. [12] and Stutzmann et al. [13].

## References


[1] Batatia, I., Kovács, D.P., Simm, G.N.C., Ortner, C., Csányi, G.: MACE: Higher Order Equivariant Message Passing Neural Networks for Fast and Accurate Force Fields (2022)

[2] Kingma, D.P., Ba, J.: Adam: A Method for Stochastic Optimization. arXiv (2017)

[3] Correa, G.B., Zhang, Y., Abreu, C.R.A., Tavares, F.W., Maginn, E.J.: Revisiting the pseudo-supercritical path method: An improved formulation for the alchemical calculation of solid–liquid coexistence. The Journal of Chemical Physics **159**(10), 104105 (2023) https://doi.org/10.1063/5.0163564

[4] Larsen, P.M., Schmidt, S., Schiøtz, J.: Robust structural identification via polyhedral template matching. Modelling and Simulation in Materials Science and Engineering **24**(5), 055007 (2016) https://doi.org/10.1088/0965-0393/24/5/055007

[5] Stukowski, A.: Visualization and analysis of atomistic simulation data with OVITO-the open visualization tool. MODELLING AND SIMULATION IN MATERIALS SCIENCE AND ENGINEERING **18**(015012) (2010) https://doi.org/10.1088/0965-0393/18/1/015012

[6] Vega, C., Sanz, E., Abascal, J.L.F., Noya, E.G.: Determination of phase diagrams via computer simulation: Methodology and applications to water, electrolytes and proteins. Journal of Physics: Condensed Matter **20**(15), 153101 (2008) https://doi.org/10.1088/0953-8984/20/15/153101

[7] Freitas, R., Asta, M., Koning, M.: Nonequilibrium free-energy calculation of solids using LAMMPS. Computational Materials Science **112**, 333–341 (2016)

[8] Tuckerman, M.E.: Statistical Mechanics: Theory and Molecular Simulation, Reprinted (with corr.) edn. Oxford Graduate Texts. Oxford Univ. Press, Oxford (2015)

[9] Bullerjahn, J.T., von Bülow, S., Heidari, M., Hénin, J., Hummer, G.: Unwrapping NPT Simulations

to Calculate Diffusion Coefficients. Journal of Chemical Theory and Computation **19**(11), 3406–3417 (2023) https://doi.org/10.1021/acs.jctc.3c00308

[10] Batatia, I., Benner, P., Chiang, Y., Elena, A.M., Kovács, D.P., Riebesell, J., Advincula, X.R., Asta, M., Avaylon, M., Baldwin, W.J., Berger, F., Bernstein, N., Bhowmik, A., Bigi, F., Blau, S.M., Cărare, V., Ceriotti, M., Chong, S., Darby, J.P., De, S., Pia, F.D., Deringer, V.L., Elijošius, R., El-Machachi, Z., Falcioni, F., Fako, E., Ferrari, A.C., Gardner, J.L.A., Gawkowski, M.J., Genreith-Schriever, A., George, J., Goodall, R.E.A., Grandel, J., Grey, C.P., Grigorev, P., Han, S., Handley, W., Heenen, H.H., Hermansson, K., Holm, C., Ho, C.H., Hofmann, S., Jaafar, J., Jakob, K.S., Jung, H., Kapil, V., Kaplan, A.D., Karimitari, N., Kermode, J.R., Kourtis, P., Kroupa, N., Kullgren, J., Kuner, M.C., Kuryla, D., Liepuoniute, G., Lin, C., Margraf, J.T., Magdău, I.-B., Michaelides, A., Moore, J.H., Naik, A.A., Niblett, S.P., Norwood, S.W., O'Neill, N., Ortner, C., Persson, K.A., Reuter, K., Rosen, A.S., Rosset, L.A.M., Schaaf, L.L., Schran, C., Shi, B.X., Sivonxay, E., Stenczel, T.K., Svahn, V., Sutton, C., Swinburne, T.D., Tilly, J., van der Oord, C., Vargas, S., Varga-Umbrich, E., Vegge, T., Vondrák, M., Wang, Y., Witt, W.C., Wolf, T., Zills, F., Csányi, G.: A Foundation Model for Atomistic Materials Chemistry (2025)

[11] Wen, T., Wang, R., Zhu, L., Zhang, L., Wang, H., Srolovitz, D.J., Wu, Z.: Specialising neural network potentials for accurate properties and application to the mechanical response of titanium. npj Computational Materials **7**(1), 1–11 (2021) https://doi.org/10.1038/s41524-021-00661-y

[12] Errandonea, D., Schwager, B., Ditz, R., Gessmann, C., Boehler, R., Ross, M.: Systematics of transition-metal melting. Physical Review B **63**(13), 132104 (2001) https://doi.org/10.1103/PhysRevB.63.132104

[13] Stutzmann, V., Dewaele, A., Bouchet, J., Bottin, F., Mezouar, M.: High-pressure melting curve of titanium. Physical Review B **92**(22), 224110 (2015) https://doi.org/10.1103/PhysRevB.92.224110
